# Supplementary material for: FLTracer: Accurate Poisoning Attack Provenance in Federated Learning
Source: arXiv:2310.13424 source file (2023-10-20)
Supplement: Supplementary file 1 [file supplement.tex]

% Supplemental material should not exceed 4 double-column pages (10 point font).
